# Supplementary material for: Multimodal Trajectory Prediction via Topological Invariance for Navigation at Uncontrolled Intersections
Source: arXiv:2011.03894 source file (2020-11-08)
Supplement: Supplementary file 1 [file supplementary.tex]

\appendix\label{sec:appendix}

\subsubsection{Rollouts \& Cost Function}

At each MPC step, the ego agent invokes the GraphNet model which generates a set of $K$ distinct multiagent trajectory predictions $\mathbf{X}^{\Lambda_{1}},\dots,\mathbf{X}^{\Lambda_{K}}$ corresponding to all modes that are possible to emerge from the current system state $X^{t}$. These predictions are spanning the space of all possible winding signatures but incorporate the constraint of the ego agent making it to its own destination $d_{i}$. They are then are fed to the MPC as rollouts to inform the control selection towards a collision-free outcome. The rollout of minimum cost is decided and its first waypoint is passed to a low-level PID controller that converts it into a control command $u_{i}^{*}$ that is immediately executed.

The cost function $J$ is defined as a weighted sum:
\begin{equation}
\begin{split}
J(\left\{\tau_{i, 1}^{t+1}, \cdots,\tau_{i, K}^{t+1}\right\}, \mathbf{X}^{t+1}) = w_{sm}J_{sm} + w_{S}J_{S} + w_{cc}J_{cc} + w_{cte}J_{cte}.
\end{split}\label{eq:cost}\mbox{,}
\end{equation}
comprising a smoothness term $J_{Sm} = \sum\limits_{t=0}^{T - 1}\gamma^{t}||v_{t+1} - v_{t}||$, information entropy cost $J_{S} = -\sum\limits_{k \in K}P(\tau_{i, k}^{t+2}, C)\log_{2}P(\tau_{i, k}^{t+2}, C)$, a collision cost $J_{cc}$, and a cross-track error term $J_{CTE}$, with $w_{sm}$, $w_{S}$, $w_{cc}$, and $w_{cte}$ as their respective weights. The collision cost $J_{cc}$ is defined as $J_{cc} = \sum\limits_{t=0}^{T}\gamma^{t}c_{t}$, where:
\begin{equation}
    c_{t} = 
    \begin{cases}
    0 & \textnormal{if}\: D_{i}(X^{t}) \geq d_{min}\\
    1 & \textnormal{else}
    \end{cases}\mbox{,}
\end{equation}
where $D_{i}$ is a distance function and $d_{min}$ is a distance threshold. To reduce the computational burden of collision-checking, we use the circle-based collision checking method by reducing the car footprint to a set of three circles covering the car volume. Any object is thus in collision with the vehicle, if its distance from the center is less than the radius.
